# Supplementary material for: ThingPot: an interactive Internet-of-Things honeypot
Source: arXiv:1807.04114 source file (2018-07-11)
Supplement: Supplementary file 1 [file appendix.tex]

\section{}
\begin{table}[!htb]
\centering
\begin{tabular}{ll}
\hline
  Count  & URL & Remark \\ 
  \hline
31607   & /api/   \\ 
% 8144 & /api/aaaaaaaaaabbbbbbbbbbccccccccccdddddddddd \\ 
2984    & /api/list/ \\ 
2910    & /         \\ 
622     & http://testp3.pospr.waw.pl/testproxy.php \\ 
% 608 & /api/aaaaaaaaaabbbbbbbbbbccccccccccdddddddddd/lights/1/state \\ 
280 & /http:/84.19.176.29:80/mysql/admin/ \\ 
275 & /http:/84.19.176.29:80/sql/php-myadmin/ \\ 
274 & /http:/84.19.176.29:80/phpmyadmin/ \\ 
274 & /http:/84.19.176.29:80/PMA2012/ \\ 
274 & /http:/84.19.176.29:80/pma2015/ \\ 
273 & /http:/84.19.176.29:80/PMA2015/ \\ 
273 & /http:/84.19.176.29:80/PMA2014/ \\ 
% 272 & /http:/84.19.176.29:80/sql/sql/ \\ 
% 272 & /http:/84.19.176.29:80/administrator/pma/ \\ 
% 272 & /http:/84.19.176.29:80/phpMyAdmin-3/ \\ 
% 94      & /manager/html& not-targeted \\ 
% 65      & /api.sfish/  & not-targeted \\ 
% 63 & /favicon.ico \\ %?????????????????
% 60 & /sfi9876.tar.bz2  & not-targeted\\ 
% 60 & /sfi9876.test      & not-targeted\\ 
% 60 & /sfi9876.xml   & not-targeted \\ 
% 60 & /sfi9876.tpl    & not-targeted \\ 
% 60 & /sfi9876.tar.gz    & not-targeted \\ 
% 60 & /sfi9876.xslt    & not-targeted \\ 
% 60 & /sfi9876.tar     & not-targeted\\ 
% 60 & /sfi9876.zip     & not-targeted\\ 
% 60 & /sfi9876.war     & not-targeted\\ 
% 60 & /sfi9876.vbs     & not-targeted\\ 
% 60 & /sfi9876.swp     & not-targeted\\ 
% 60 & /sfi9876.xsl     & not-targeted\\ 
% 60 & /sfi9876.ws     & not-targeted\\ 
% 60 & /sfi9876.txt     & not-targeted\\ 
% 60 & /sfi9876.temp     & not-targeted\\ 
% 60 & /sfi9876.xls     & not-targeted\\ 
% 60 & /sfi9876.yml     & not-targeted\\ 
% 60 & /sfi9876.tgz     & not-targeted\\ 
% 60 & /sfi9876.trace     & not-targeted\\ 
% 60 & /sfi9876.tmp     & not-targeted\\ 
% 60 & /sfi9876.vb     & not-targeted\\ 
\hline
\end{tabular}
\caption{Top 11 URLs from HTTP requests taken from the proxy logs}
\label{tab-proxy-http-url}
\end{table}
\begin{table}[ht]
\centering
\begin{tabular}{p{15pt}p{360pt}p{60pt}}
\hline
  Count  & Request & Remark \\ 
  \hline
31 & "\@\backslash x00\backslash x00\backslash x00B\backslash xA4" \\ 
8 & "OPTIONS / RTSP/1.0" & not targeted\\ 

8 & "Gh0st\backslash xAD\backslash x00\backslash x00\backslash x00\backslash xE0\backslash x00\backslash x00\backslash x00x\backslash x9CKS``\backslash x98\backslash xC3\backslash xC0\backslash xC0\backslash xC0\backslash x06

\backslash xC4\backslash x8C@\backslash xBCQ\backslash x96\backslash x81\backslash x81\backslash x09H\backslash x07\backslash xA7\backslash x16\backslash x95e\&\backslash xA7\ast\backslash x04\$\&g+\backslash x182\backslash x94\backslash xF6\backslash xB000\backslash xAC\backslash xA8rc\backslash x00\backslash x01\backslash x11\backslash xA0\backslash x82\backslash x1F\backslash x5C`\&\backslash x83\backslash xC7K7

\backslash x86\backslash x19\backslash xE5n\backslash x0C9\backslash x95n\backslash x0C;\backslash x84\backslash x0F3\backslash xAC\backslash xE8sch\backslash xA8^\backslash xCF4'J\backslash x97\backslash xA9\backslash x82

\backslash xE30\backslash xC3\backslash x91h]\&\backslash x90\backslash xF8\backslash xCE\backslash x97S\backslash xCBA4L?2=\backslash xE1\backslash xC4\backslash x92\backslash x86\backslash x0B@\backslash xF5`

\backslash x0CT\backslash x1F\backslash xAE\backslash xAF]" \\ 
8 & "\backslash x04\backslash x01\backslash x00P\backslash xC0c\backslash x F660\backslash x00" \\ 
8 & "OPTIONS / HTTP/1.0" \\ 
7 & "USER test +iw test :Test Wuz Here" \\ 

5 & "@\backslash x00\backslash x00\backslash x00\backslash x00Z\backslash xE6\backslash xCA\backslash x22BX\backslash x1C\backslash x86\-\backslash x9B\backslash xB0#\backslash xB2N\backslash xF6(\backslash x13o\backslash xF5

\backslash xB03Xo\backslash xC0.\backslash x  A6W\backslash xB0d\backslash xD7Qsf\backslash x D1\backslash xA1\backslash x0C\backslash xB0V\backslash xC32.\backslash xB3@\backslash x

0BI\backslash x01\backslash x00\backslash xF6\backslash x867\backslash x9A+\backslash x13\backslash x02I!?[\backslash x9D=\backslash x08\backslash xE4N" \\ 
5 & "FOO /FOO-sfi9876 HTTP/1.1" \\ 
4 & "" \\ 
4 & "\backslash x05\backslash x02\backslash x00\backslash x02" \\
\hline
\end{tabular}% TOTAL????????????????????
\caption{Top 10 non HTTP requests taken from the proxy logs}
\label{tab-proxy-nohttp-request}
\end{table}

% \begin{table}[ht]
% \centering
% \begin{tabular}{ll}
% \hline
%   Count  & URL  \\ 
%   \hline
% 2910 & / \\ 
% 622 & http://testp3.pospr.waw.pl/testproxy.php \\ 
% 94 & /manager/html \\ 
% 65 & /api.sfish/ \\ 
% 60 & /sfi9876.xslt \\ 
% 60 & /sfi9876.tpl \\ 
% 60 & /sfi9876.tar.gz \\ 
% 60 & /sfi9876.tar \\ 
% 60 & /sfi9876.zip \\ 
% 60 & /sfi9876.war \\ 
% 60 & /sfi9876.test \\ 
% 60 & /sfi9876.tar.bz2 \\ 
% 60 & /sfi9876.xml \\ 
% 60 & /sfi9876.trace \\ 
% 60 & /sfi9876.tgz \\ 
% 60 & /sfi9876.tmp \\ 
% 60 & /sfi9876.vb \\ 
% 60 & /sfi9876.xsl \\ 
% 60 & /sfi9876.vbs \\ 
% 60 & /sfi9876.swp \\ 
% 60 & /sfi9876.yml \\ 
% 60 & /sfi9876.ws \\ 
% 60 & /sfi9876.temp \\ 
% 60 & /sfi9876.txt \\ 
% 60 & /sfi9876.xls \\ 
% \hline
% \end{tabular}% TOTAL????????????????????????????????
% \caption{Top 26 HTTP URLs not started with "/api" taken from the proxy logs}
% \label{tab-proxy-http-urls-others}
% \end{table}

\begin{table}[ht]
\centering
\begin{tabular}{lll}
\hline
  Count  & IP & TOR? \\ 
  \hline
1338 & 104.223.123.98 & Yes\\ 
1060 & 192.42.116.16 & Yes\\ 
889 & 89.234.157.254 & Yes\\ 
736 & 79.172.193.32 & Yes\\ 
717 & 204.85.191.30 & Yes\\ 
694 & 94.242.246.24 & Yes\\ 
671 & 94.242.246.23 & Yes\\ 
669 & 91.223.82.156 & Yes\\ 
663 & 5.254.79.66 & Yes\\ 
649 & 78.109.23.1 & Yes\\ 
610 & 176.126.252.11& Yes \\ 
572 & 216.218.222.13 & Yes\\ 
565 & 163.172.212.115 & Yes\\ 
564 & 185.170.42.4& Yes \\ 
555 & 196.54.55.13 & No\\ %shooter
550 & 109.163.234.9 & Yes\\ % shooter
532 & 193.90.12.88 & Yes\\ % shooter
521 & 185.170.41.8 & Yes\\ % shooter
499 & 79.137.67.116 & Yes\\ % shooter
479 & 163.172.67.180 & Yes\\ % shooter
\hline
\end{tabular}
\caption{Top 20 source IP addresses from all requests taken from the api logs}
\label{tab-api-remoteips}
\end{table}

\begin{table}[ht]
\centering
\begin{tabular}{ll}
\hline
  Count  & IP   \\ 
  \hline
20 & 193.70.95.180 \\ 
18 & 164.52.7.132 \\ 
15 & 220.181.159.73 \\ 
12 & 47.203.93.185 \\ 
8 & 66.240.205.34 \\ 
7 & 93.115.95.207 \\ 
6 & 180.97.106.162 \\ 
5 & 110.90.95.163 \\ 
4 & 185.100.87.246 \\ 
4 & 208.100.26.229 \\ 
3 & 72.11.140.74 \\ 
\hline
\end{tabular}% TOTAL????????????????????????????????
\caption{Top 10 IP address of the non HTTP requests taken from the proxy logs}
\label{tab-proxy-nonhttp-sourceip}
\end{table}

\begin{table}[ht]
\centering
\begin{tabular}{ll}
\hline
  Count  & autonomous system number (ASN)  \\ 
  \hline
24 & 36351 \\ 
23 & 4134 \\ 
23 & 12876 \\ 
23 & 16276 \\ 
17 & 28573 \\ 
13 & 15169 \\ 
9 & 60781 \\ 
9 & 4837 \\ 
9 & 14061 \\ 
8 & 62567 \\ 
8 & 63949 \\ 
8 & 3223 \\ 
7 & 8100 \\ 
7 & 23650 \\ 
6 & 23724 \\ 
6 & 10439 \\ 
6 & 16509 \\ 
6 & 36375 \\ 
6 & 42570 \\ 
6 & 3462 \\ 
\hline
\end{tabular}
\caption{Top 20 countries that IP addresses is located}
\label{tab-proxy-sourceip-asn}
\end{table}  % appendix??
\begin{table}[ht]
\centering
\begin{tabular}{lp{80pt}p{220pt}}
\hline
  Count  & Regional Internet Registry (RIR) & Remark  \\ 
  \hline
258 & ripencc & Réseaux IP Européens Network Coordination Centre (RIPE NCC) \cite{reipncc} for Europe, Russia, the Middle East, and Central Asia\\ 
142 & arin & American Registry for Internet Numbers (ARIN) \cite{arin} for the United States, Canada, several parts of the Caribbean region, and Antarctica. \\ 
110 & apnic & Asia-Pacific Network Information Centre (APNIC) \cite{apnic} for Asia, Australia, New Zealand, and neighboring countries\\ 
31 & lacnic& Latin America and Caribbean Network Information Centre (LACNIC) \cite{lacnic} for Latin America and parts of the Caribbean region \\ 
16 & afrinic & African Network Information Center (AFRINIC) \cite{afrinic} for Africa \\ 
3 & & no RIR is recorded \\ 

\hline
\end{tabular}
\caption{The RIR of the IP addresses}
\label{tab-proxy-sourceip-rir}
\end{table}

\begin{table}[ht]
\centering
\begin{tabular}{p{40pt}l}
\hline
  Count  & User Agent  \\ 
  \hline
1328204 & "-" \\ 
31567 & "shooter" \\ 
20162 & "Mozilla/5.0 SF/2.10b" \\ 
2984 & "botlight" \\ 
2378 & "000modscan" \\ 
1867 & "httpget" \\ 
831 & "Mozilla/5.0 (Windows NT 10.0; WOW64; Trident/7.0; rv:11.0) like Gecko" \\ 
622 & "Mozilla/5.0 (Windows NT 5.1; rv:32.0) Gecko/20100101 Firefox/31.0" \\ 
607 & "0000modscan" \\ 
313 & "Mozilla/5.0 (Windows NT 6.1; WOW64; Trident/7.0; rv:11.0) like Gecko" \\ 
% 275 & "Mozilla/5.0 (Macintosh; Intel Mac OS X 10.11; rv:47.0) Gecko/20100101 Firefox/47.0" \\ 
% 236 & "Mozilla/5.0 (X11; U; Linux i686; en-US; rv:1.9.0.2) Gecko/2008092809 Gentoo Firefox/3.0.2" \\ 
% 186 & "Mozilla/5.0 (Windows NT 6.3; WOW64; Trident/7.0; rv:11.0) like Gecko" \\ 
% 158 & "Mozilla/5.0 (Windows NT 6.3; WOW64; Trident/7.0; Touch; rv:11.0) like Gecko" \\ 
% 154 & "Mozilla/5.00 (Nikto/2.1.5) (Evasions:None) (Test:map\_codes)" \\ 
% 148 & "Mozilla/5.0 (X11; Linux x86\_64) AppleWebKit/537.36 (KHTML, like Gecko) Chrome

% /59.0.3071.115 Safari/537.36" \\ 
% 110 & "Mozilla/5.0 (X11; Linux x86\_64) AppleWebKit/537.36 (KHTML, like Gecko) Chrome

% /58.0.3029.110 Safari/537.36" \\ 
% 103 & "Mozilla/5.0 (Windows NT 10.0; WOW64; Trident/7.0; Touch; LCJB; rv:11.0) like Gecko" \\ 
% 85 & "curl/7.52.1" \\ 
% 83 & "Mozilla/5.0 zgrab/0.x" \\ 
\hline
\end{tabular}% TOTAL????????????????????????????????
\caption{Top 20 user agents from HTTP requests taken from the proxy logs}
\label{tab-proxy-http-urls-useragent}
\end{table}

\begin{table}[ht]
\centering
\begin{tabular}{p{40pt}p{360pt}}
\hline
  Count  & User Agent  \\ 
  \hline
225 & "-" \\ 
47 & "Mozilla/5.0 SF/2.10b" \\ 
1 & "Mozilla/5.0 (Macintosh; Intel Mac OS X 10\_6\_8) AppleWebKit/536.5 (KHTML, like Gecko)

Chrome/19.0.1084.56 Safari/536.5" \\ 
1 & "Mozilla/5.0 (compatible; MSIE 8.0; MSIE 9.0; Windows NT 6.0; Trident/4.0; InfoPath.1; SV1; .NET CLR 3.8.36217; WOW64; en-US)" \\ 
1 & "curl/7.53.1" \\ 
1 & "Mozilla/5.0 (compatible; Googlebot/2.1; +http://www.google.com/bot.html)" \\ 
\hline
\end{tabular}
\caption{User Agents of the non HTTP requests taken from the proxy logs}%???????
\label{tab-proxy-nonhttp-useragent}
\end{table}

\begin{table}[ht]
\centering
\begin{tabular}{p{40pt}p{360pt}}
\hline
  Count  & User Agent  \\ 
  \hline
1327485 & "-" \\ 
31567 & "shooter" \\ 
2984 & "botlight" \\ 
2378 & "000modscan" \\ 
1867 & "httpget" \\ 
606 & "0000modscan" \\ 
154 & "Mozilla/5.00 (Nikto/2.1.5) (Evasions:None) (Test:map\_codes)" \\ 
107 & "Mozilla/5.0 (X11; Linux x86\_64) AppleWebKit/537.36 (KHTML, like Gecko) Chrome

/59.0.3071.115 Safari/537.36" \\ 
98 & "Mozilla/5.0 SF/2.10b" \\ 
85 & "curl/7.52.1" \\  
\hline
\end{tabular}% TOTAL????????????????????????????????
\caption{Top 10 User Agents from the requests started with "/api" taken from the proxy logs}
\label{tab-proxy-http-urls-api-useragent}
\end{table}

\begin{table}[ht]
\centering
\begin{tabular}{ll}
\hline
  Count  & User Agent  \\ 
  \hline
20064 & "Mozilla/5.0 SF/2.10b" \\ 
831 & "Mozilla/5.0 (Windows NT 10.0; WOW64; Trident/7.0; rv:11.0) like Gecko" \\ 
719 & "-" \\ 
622 & "Mozilla/5.0 (Windows NT 5.1; rv:32.0) Gecko/20100101 Firefox/31.0" \\ 
313 & "Mozilla/5.0 (Windows NT 6.1; WOW64; Trident/7.0; rv:11.0) like Gecko" \\ 
275 & "Mozilla/5.0 (Macintosh; Intel Mac OS X 10.11; rv:47.0) Gecko/20100101 Firefox/47.0" \\ 
236 & "Mozilla/5.0 (X11; U; Linux i686; en-US; rv:1.9.0.2) Gecko/2008092809 Gentoo Firefox/3.0.2" \\ 
186 & "Mozilla/5.0 (Windows NT 6.3; WOW64; Trident/7.0; rv:11.0) like Gecko" \\ 
158 & "Mozilla/5.0 (Windows NT 6.3; WOW64; Trident/7.0; Touch; rv:11.0) like Gecko" \\ 
103 & "Mozilla/5.0 (Windows NT 10.0; WOW64; Trident/7.0; Touch; LCJB; rv:11.0) like Gecko" \\ 
\hline
\end{tabular}
\caption{Top 10 user agents from URLs not started with "/api" taken from the proxy logs}
\label{tab-proxy-http-urls-others-useragent}
\end{table}

\begin{table}[ht]
\centering
\begin{tabular}{lp{160pt}p{200pt}}
\hline
  Count  & Referer & Remarks \\ 
  \hline
20 & https://proxyradar.com/ & It has a list of working open proxies. \\ 
13 & http://84.19.177.29:80 \\ 
12 & http://84.19.176.29/phpmyadmin \\ 
11 & http://84.19.176.29:80 \\ 
10 & http://vegenis.servequake.com/ & Valid URL to reach the node of the honeypot.\\ 
6 & http://84.19.177.29/phpmyadmin \\ 
5 & http://84.19.177.29/ \\ 
5 & http://morris.jusanet.org/api/belkin/

wemo/af3bdcebd800931357951db376

e0dad7 & This is a very specific URL that is targetting to Belkin Wemo.\\ 
4 & http://84.19.176.29/ & Valid URL to reach the node of the honeypot.\\ 
4 & http://morris.jusanet.org/ & Valid URL to reach the node of the honeypot.\\ 
3 & http://84.19.177.29/api/ & Valid URL to reach the node of the honeypot.\\ 
2 & http://84.19.177.29:80/ & Valid URL to reach the node of the honeypot. \\ 
2 & http://www.google.com/search?hl=ru

\&q=free+proxy+checker\&sourceid=na

vclient-ff\&ie=UTF-8 \\ 
2 & http://www.google.com/search \\ 
1 & http://84.19.176.29/api/ & Valid URL to reach the node of the honeypot. \\ 
1 & http://84.19.177.29/phpmyadmin/in

dex.php \\ 
1 & http://84.19.177.29/db/phpMyAdmin-3/ \\ 
1 & http://84.19.176.29:80/ & Valid URL to reach the node of the honeypot. \\ 
1 & http://84.19.176.29:80/shell?\%65\%63

\%68\%6F\%20\%63\%61\%6E\%6C\%61\%6E

\%67 & It could be decoded as "http://84.19.176.29:80/shell?echo canlang"  This URL is reported on the \textit{www.abuseipdb.com}.\\ 
1 & http://84.19.177.29/pma/ \\ 
\hline
\end{tabular}
\caption{Referers taken from the API logs}
\label{tab-api-referers}
\end{table}
